# Supplementary material for: The Dawn of GUI Agent: A Preliminary Case Study with Claude 3.5 Computer Use
Source: arXiv:2411.10323 source file (2024-11-15)
Supplement: Supplementary file 1 [file A-placeholder.tex]

\section{Appendix}
\subsection{Prompt templates}
\label{sec:appendix}
